# Supplementary material for: Knowledge Base Completion Meets Transfer Learning
Source: arXiv:2108.13073 source file (2021-08-30)
Supplement: Supplementary file 1 [file appendix.pdf]

## A Metrics

This section contains a formal description of the metrics that were used to score the models. Let  $\langle h, r, t \rangle$  be some test triple. Given  $\langle h, r, ? \rangle$ , the model is used to rank all entities in the knowledge base from the most suitable to the least suitable tail, so that the entity no. 1 is the most likely tail according to the model. All ranks are reported in the “filtered setting”, which means that all other known correct answers, other than  $t$ , are removed from this list to reduce noise. Let  $r_t$  be the position or *rank* of the correct tail in this list. In ReVerb20K and ReVerb45K, there may be entities from the same cluster as  $t$ , equivalent to  $t$ . In this case,  $r_t$  is the lowest of their ranks. The *reciprocal rank* of an example is then defined as  $\frac{1}{r_t}$ . The same process is repeated with the input  $\langle ?, r, t \rangle$  and the head entity.

The *mean rank (MR)* of the model is the average of all ranks across all test examples, both heads and tails. The *mean reciprocal rank (MRR)* is the average of all reciprocal ranks, both heads and tails. The *Hits@N* metric tells us how often the rank was smaller or equal to  $N$ . The related literature most commonly uses 1, 3, and 10 for values of  $N$ , however, 5, 30, and 50 are also occasionally reported.

## B Detailed Experimental Setup

Following Ruffinelli et al. (2020), we use 1-N scoring for negative sampling and cross-entropy loss for all models. The Adam optimizer (Kingma and Ba, 2015) was used to train the network. We follow Dettmers et al. (2018) and Balažević et al. (2019) with the placement of batch norm and dropout in ConvE and TuckER, respectively, however, we simplify the setup by always setting all dropout rates to the same value to reduce the hyperparameter space. To find the best hyperparameters, grid search is used for all experiments to exhaustively compare all options. Despite numerous simplifications, we find that our re-implementations of the baselines (non-pre-trained NoEncoder models) perform comparable to the original reported values. The experiments were performed on a DGX-1 cluster, using one Nvidia V100 GPU per experiment.

**Pre-training setup.** Pre-training was only done with GRU encoders, as discussed in Section 2.1. Due to the large number of entities in the pre-training set, 1-N sampling is only performed with negative examples from the same batch, and batches of size 4096 were used, follow-

ing Broscheit et al. (2020). The learning rate was selected from  $\{1 \cdot 10^{-4}, 3 \cdot 10^{-4}\}$ , while the dropout rate was selected from  $\{0.2, 0.3\}$  for ConvE and  $\{0.3, 0.4\}$  for TuckER. For 5\*E, the dropout rate was not used, but N3 regularization was (Lacroix et al., 2018), its weight selected from  $\{0.1, 0.03\}$ . For TuckER, models with embedding dimensions 100, 200, and 300 were trained. We saved the best model of each dimension for fine-tuning. For ConvE, models with embedding dimensions 300 and 500 were trained, and the best model for each dimension was saved for fine-tuning. Following Gupta et al. (2019), we use a single 2d convolution layer with 32 channels and  $3 \times 3$  kernel size. When the dimension of entities and relations is 300, they were reshaped into  $15 \times 20$  inputs, while the  $20 \times 25$  input shapes were used for the 500-dimensional embeddings. For 5\*E, models with embedding dimensions 200 and 500 were trained, and the best model for each dimension was saved for fine-tuning. Following Broscheit et al. (2020), we trained each model for 100 epochs. Testing on the validation set is performed each 20 epochs, and the model with the best overall mean reciprocal rank (MRR) is selected.

**Fine-tuning setup.** Fine-tuning is performed in the same way as the pre-training, however, the models were trained for 500 epochs, and a larger hyperparameter space was considered. More specifically, the learning rate was selected from  $\{3 \cdot 10^{-5}, 1 \cdot 10^{-4}, 3 \cdot 10^{-4}\}$ . The dropout rate was selected from  $\{0.2, 0.3\}$  for ConvE and  $\{0.3, 0.4\}$  for TuckER. The weight of N3 regularization for the 5\*E models was selected from  $\{0.3, 0.1, 0.03\}$ . The batch size was selected from  $\{512, 1024, 2048, 4096\}$ . The same embedding dimensions as for pre-training were considered.

## C Full Results

This appendix contains detailed information on the best performance of all models. Table 6 contains the detailed information on the performance of the best models both on validation and test sets of the datasets. Table 7 includes information on the best hyperparameter setups and approximate training times. Note that the given times are approximate and are strongly affected by the selection of the hyperparameters as well as external factors.

|            |              | OlpBench validation |             |             |             |             |             |             |             | OlpBench test |             |             |             |             |             |             |             |
|------------|--------------|---------------------|-------------|-------------|-------------|-------------|-------------|-------------|-------------|---------------|-------------|-------------|-------------|-------------|-------------|-------------|-------------|
| Model      | Pre-trained? | MR                  | MRR         | H@1         | H@3         | H@5         | H@10        | H@30        | H@50        | MR            | MRR         | H@1         | H@3         | H@5         | H@10        | H@30        | H@50        |
| GRU_TUCKER | no           | <b>55.6K</b>        | .058        | .0.033      | .060        | .076        | .104        | .163        | .195        | <b>57.2K</b>  | .053        | .029        | .054        | .070        | .097        | .155        | .189        |
| GRU_CONVE  | no           | 57.6K               | .047        | .025        | .048        | .063        | .090        | .147        | .179        | <b>57.2K</b>  | .045        | .022        | .047        | .060        | .086        | .140        | .173        |
| GRU_5*E    | no           | 60.1K               | <b>.060</b> | <b>.034</b> | <b>.061</b> | <b>.078</b> | <b>.109</b> | <b>.171</b> | <b>.205</b> | 59.9K         | <b>.055</b> | <b>.030</b> | <b>.056</b> | <b>.075</b> | <b>.101</b> | <b>.160</b> | <b>.194</b> |

  

|                  |              | ReVerb20K validation |             |             |             |             |             |             |             | ReVerb20K test |             |             |             |             |             |             |             |
|------------------|--------------|----------------------|-------------|-------------|-------------|-------------|-------------|-------------|-------------|----------------|-------------|-------------|-------------|-------------|-------------|-------------|-------------|
| Model            | Pre-trained? | MR                   | MRR         | H@1         | H@3         | H@5         | H@10        | H@30        | H@50        | MR             | MRR         | H@1         | H@3         | H@5         | H@10        | H@30        | H@50        |
| NoENCODER_TUCKER | no           | 2532                 | .196        | .160        | .207        | .230        | .265        | .318        | .352        | 2611           | .196        | .157        | .212        | .236        | .267        | .332        | .362        |
|                  | yes          | 354                  | .367        | .283        | .400        | .457        | .529        | .646        | .702        | 303            | .367        | .295        | .412        | .466        | .540        | .659        | .714        |
| NoENCODER_CONVE  | no           | 1376                 | .279        | .233        | .301        | .329        | .364        | .423        | .458        | 1419           | .282        | .227        | .308        | .338        | .380        | .442        | .475        |
|                  | yes          | 292                  | .392        | .312        | .423        | .477        | .546        | .658        | .706        | 227            | .400        | .313        | .440        | .491        | .568        | .680        | .729        |
| NoENCODER_5*E    | no           | 2213                 | .230        | .180        | .243        | .279        | .325        | .421        | .468        | 2301           | .228        | .174        | .243        | .278        | .334        | .429        | .473        |
|                  | yes          | 773                  | .249        | .194        | .263        | .299        | .353        | .466        | .528        | 780            | .249        | .191        | .264        | .302        | .363        | .471        | .532        |
| GRU_TUCKER       | no           | 646                  | .344        | .277        | .366        | .409        | .470        | .564        | .609        | 598            | .357        | .283        | .391        | .434        | .493        | .594        | .639        |
|                  | yes          | 283                  | .386        | .305        | .416        | .465        | .543        | .660        | .707        | 245            | .397        | .315        | .429        | .485        | .558        | .674        | .720        |
| GRU_CONVE        | no           | 333                  | .377        | .305        | .405        | .447        | .516        | .635        | .683        | 334            | .387        | .305        | .421        | .471        | .540        | .648        | .690        |
|                  | yes          | <b>229</b>           | .397        | .317        | .428        | .477        | .554        | .671        | .726        | <b>184</b>     | .409        | .326        | .442        | .499        | .573        | .687        | .737        |
| GRU_5*E          | no           | 430                  | .379        | .302        | .411        | .454        | .523        | .639        | .685        | 395            | .390        | .311        | .422        | .475        | .546        | .650        | .697        |
|                  | yes          | 243                  | <b>.404</b> | <b>.318</b> | <b>.440</b> | <b>.492</b> | <b>.569</b> | <b>.690</b> | <b>.747</b> | 202            | <b>.417</b> | <b>.330</b> | <b>.455</b> | <b>.512</b> | <b>.586</b> | <b>.701</b> | <b>.748</b> |

  

|                  |              | ReVerb45K validation |             |             |             |             |             |             |             | ReVerb45K test |             |             |             |             |             |             |             |
|------------------|--------------|----------------------|-------------|-------------|-------------|-------------|-------------|-------------|-------------|----------------|-------------|-------------|-------------|-------------|-------------|-------------|-------------|
| Model            | Pre-trained? | MR                   | MRR         | H@1         | H@3         | H@5         | H@10        | H@30        | H@50        | MR             | MRR         | H@1         | H@3         | H@5         | H@10        | H@30        | H@50        |
| NoENCODER_TUCKER | no           | 5097                 | .094        | .077        | .097        | .109        | .126        | .160        | .177        | 5135           | .103        | .088        | .106        | .116        | .131        | .164        | .182        |
|                  | yes          | 839                  | .305        | .228        | .335        | .386        | .453        | .559        | .610        | 780            | .299        | .220        | .332        | .386        | .453        | .557        | .607        |
| NoENCODER_CONVE  | no           | 2741                 | .235        | .180        | .262        | .293        | .336        | .406        | .436        | 2690           | .232        | .179        | .256        | .288        | .333        | .400        | .434        |
|                  | yes          | 632                  | .353        | .274        | .384        | .438        | .506        | .611        | .662        | 666            | .345        | .267        | .378        | .432        | .500        | .601        | .644        |
| NoENCODER_5*E    | no           | 3653                 | .148        | .116        | .151        | .174        | .210        | .289        | .324        | 3460           | .152        | .123        | .152        | .174        | .212        | .289        | .327        |
|                  | yes          | 3233                 | .187        | .151        | .195        | .222        | .258        | .320        | .349        | 3279           | .189        | .153        | .198        | .224        | .261        | .325        | .357        |
| GRU_TUCKER       | no           | 1386                 | .304        | .242        | .330        | .369        | .423        | .504        | .545        | 1398           | .302        | .242        | .323        | .365        | .420        | .506        | .546        |
|                  | yes          | 761                  | .336        | .263        | .368        | .413        | .473        | .570        | .613        | 706            | .331        | .258        | .359        | .412        | .477        | .575        | .618        |
| GRU_CONVE        | no           | 776                  | .351        | .273        | .387        | .437        | .501        | .593        | .631        | 824            | .343        | .268        | .374        | .424        | .488        | .584        | .626        |
|                  | yes          | <b>584</b>           | .364        | .285        | .400        | .452        | .518        | .620        | .665        | 600            | .357        | .277        | .393        | .444        | .509        | .607        | .651        |
| GRU_5*E          | no           | 843                  | .362        | .287        | .394        | .446        | .511        | .607        | .649        | 836            | .357        | .278        | .394        | .443        | .508        | .605        | .647        |
|                  | yes          | 603                  | <b>.385</b> | <b>.305</b> | <b>.421</b> | <b>.474</b> | <b>.542</b> | <b>.642</b> | <b>.683</b> | <b>596</b>     | <b>.382</b> | <b>.302</b> | <b>.416</b> | <b>.467</b> | <b>.537</b> | <b>.636</b> | <b>.676</b> |

  

|                  |              | FB15K237 validation |             |             |             |             |             |             |             | FB15K237 test |             |             |             |             |             |             |             |
|------------------|--------------|---------------------|-------------|-------------|-------------|-------------|-------------|-------------|-------------|---------------|-------------|-------------|-------------|-------------|-------------|-------------|-------------|
| Model            | Pre-trained? | MR                  | MRR         | H@1         | H@3         | H@5         | H@10        | H@30        | H@50        | MR            | MRR         | H@1         | H@3         | H@5         | H@10        | H@30        | H@50        |
| NoENCODER_TUCKER | no           | 160                 | .366        | .276        | .399        | .464        | .547        | .675        | .727        | 166           | .358        | .265        | .393        | .458        | .545        | .669        | .725        |
|                  | yes          | 142                 | <b>.369</b> | <b>.277</b> | <b>.403</b> | <b>.468</b> | <b>.555</b> | <b>.680</b> | <b>.732</b> | 151           | <b>.363</b> | <b>.269</b> | <b>.398</b> | <b>.464</b> | <b>.550</b> | <b>.678</b> | <b>.733</b> |
| NoENCODER_CONVE  | no           | 200                 | .326        | .238        | .356        | .419        | .508        | .634        | .690        | 212           | .320        | .230        | .351        | .417        | .504        | .634        | .690        |
|                  | yes          | 189                 | .332        | .242        | .363        | .428        | .513        | .647        | .703        | 200           | .325        | .233        | .355        | .421        | .510        | .645        | .703        |
| NoENCODER_5*E    | no           | 144                 | .358        | .267        | .393        | .456        | .542        | .670        | .723        | 152           | .353        | .260        | .389        | .454        | .539        | .666        | .721        |
|                  | yes          | <b>137</b>          | .362        | .270        | .398        | .462        | .548        | .672        | .727        | <b>143</b>    | .357        | .264        | .393        | .459        | .544        | .670        | .727        |
| GRU_TUCKER       | no           | <b>137</b>          | .355        | .262        | .391        | .454        | .539        | .671        | .724        | 144           | .350        | .256        | .386        | .451        | .538        | .666        | .723        |
|                  | yes          | <b>137</b>          | .357        | .264        | .393        | .454        | .542        | .670        | .726        | <b>143</b>    | .354        | .260        | .391        | .453        | .538        | .668        | .724        |
| GRU_CONVE        | no           | 161                 | .340        | .249        | .372        | .433        | .521        | .653        | .708        | 166           | .334        | .242        | .368        | .431        | .519        | .650        | .705        |
|                  | yes          | 151                 | .331        | .241        | .361        | .423        | .515        | .652        | .708        | 157           | .327        | .237        | .359        | .422        | .513        | .646        | .704        |
| GRU_5*E          | no           | 145                 | .351        | .256        | .387        | .453        | .540        | .669        | .725        | 150           | .345        | .249        | .380        | .449        | .536        | .667        | .725        |
|                  | yes          | 143                 | .351        | .257        | .386        | .451        | .537        | .667        | .722        | 145           | .348        | .254        | .384        | .450        | .536        | .666        | .720        |

  

|                  |              | WN18RR validation |             |             |             |             |             |             |             | WN18RR test |             |             |             |             |             |             |             |
|------------------|--------------|-------------------|-------------|-------------|-------------|-------------|-------------|-------------|-------------|-------------|-------------|-------------|-------------|-------------|-------------|-------------|-------------|
| Model            | Pre-trained? | MR                | MRR         | H@1         | H@3         | H@5         | H@10        | H@30        | H@50        | MR          | MRR         | H@1         | H@3         | H@5         | H@10        | H@30        | H@50        |
| NoENCODER_TUCKER | no           | 3701              | .469        | .437        | .483        | .499        | .524        | .571        | .595        | 4097        | .468        | .435        | .483        | .502        | .528        | .576        | .595        |
|                  | yes          | 3332              | .470        | .439        | .479        | .500        | .529        | .583        | .604        | 3456        | .467        | .434        | .480        | .500        | .529        | .583        | .604        |
| NoENCODER_CONVE  | no           | 6337              | .429        | .403        | .437        | .455        | .479        | .512        | .530        | 6455        | .429        | .404        | .440        | .455        | .479        | .512        | .530        |
|                  | yes          | 5678              | .433        | .407        | .442        | .460        | .483        | .523        | .542        | 5793        | .435        | .408        | .444        | .461        | .486        | .527        | .545        |
| NoENCODER_5*E    | no           | 2527              | <b>.492</b> | <b>.450</b> | <b>.505</b> | <b>.531</b> | .574        | .649        | <b>.680</b> | <b>2450</b> | <b>.492</b> | .448        | <b>.507</b> | <b>.534</b> | <b>.583</b> | <b>.652</b> | .680        |
|                  | yes          | 2576              | <b>.492</b> | <b>.450</b> | .501        | .528        | <b>.575</b> | <b>.651</b> | <b>.680</b> | 2636        | <b>.492</b> | <b>.450</b> | .504        | .533        | .582        | <b>.652</b> | <b>.683</b> |
| GRU_TUCKER       | no           | 3201              | .456        | .428        | .464        | .484        | .506        | .553        | .574        | 3262        | .456        | .429        | .465        | .483        | .505        | .551        | .573        |
|                  | yes          | 2637              | .457        | .422        | .469        | .490        | .523        | .579        | .609        | 2790        | .455        | .418        | .469        | .494        | .524        | .577        | .600        |
| GRU_CONVE        | no           | 4376              | .431        | .407        | .439        | .456        | .477        | .518        | .538        | 4474        | .428        | .402        | .438        | .455        | .474        | .512        | .533        |
|                  | yes          | 5983              | .400        | .376        | .410        | .422        | .444        | .475        | .493        | 6128        | .399        | .375        | .409        | .423        | .441        | .473        | .491        |
| GRU_5*E          | no           | <b>2444</b>       | .456        | .418        | .463        | .492        | .533        | .598        | .629        | 2545        | .452        | .413        | .462        | .489        | .527        | .595        | .629        |
|                  | yes          | 2971              | .426        | .388        | .440        | .464        | .494        | .548        | .575        | 3068        | .420        | .379        | .437        | .459        | .488        | .547        | .573        |

Table 6: Full results on both validation and test set of all datasets. In addition to the metrics reported in the paper, we also report H@N for  $N \in \{1, 3, 5, 10, 30, 50\}$ , which appeared in related work. The best value in each column is written in **bold**.

| Model      | Pre-trained? | dimension | learning rate     | OlpBench |         |           |         |
|------------|--------------|-----------|-------------------|----------|---------|-----------|---------|
|            |              |           |                   | batch    | dropout | N3 weight | time    |
| GRU_TUCKER | no           | 300       | $1 \cdot 10^{-4}$ | 4096     | 0.3     | –         | 5 days  |
| GRU_CONVE  | no           | 500       | $1 \cdot 10^{-4}$ | 4096     | 0.2     | –         | 5 days  |
| GRU_5★E    | no           | 500       | $1 \cdot 10^{-4}$ | 4096     | –       | 0.03      | 12 days |

  

| Model            | Pre-trained? | dimension | learning rate     | ReVerb20K |         |           |        |
|------------------|--------------|-----------|-------------------|-----------|---------|-----------|--------|
|                  |              |           |                   | batch     | dropout | N3 weight | time   |
| NoENCODER_TUCKER | no           | 300       | $3 \cdot 10^{-5}$ | 512       | 0.4     | –         | 30 min |
|                  | yes          | 300       | $3 \cdot 10^{-4}$ | 512       | 0.3     | –         | 30 min |
| NoENCODER_CONVE  | no           | 300       | $3 \cdot 10^{-4}$ | 1024      | 0.3     | –         | 30 min |
|                  | yes          | 500       | $1 \cdot 10^{-4}$ | 512       | 0.2     | –         | 30 min |
| NoENCODER_5★E    | no           | 200       | $1 \cdot 10^{-3}$ | 512       | –       | 0.3       | 30 min |
|                  | yes          | 500       | $3 \cdot 10^{-4}$ | 512       | –       | 0.03      | 30 min |
| GRU_TUCKER       | no           | 300       | $3 \cdot 10^{-3}$ | 1024      | 0.4     | –         | 30 min |
|                  | yes          | 300       | $3 \cdot 10^{-5}$ | 2048      | 0.4     | –         | 30 min |
| GRU_CONVE        | no           | 300       | $3 \cdot 10^{-5}$ | 512       | 0.3     | –         | 30 min |
|                  | yes          | 500       | $3 \cdot 10^{-5}$ | 512       | 0.3     | –         | 30 min |
| GRU_5★E          | no           | 200       | $3 \cdot 10^{-4}$ | 2048      | –       | 0.1       | 30 min |
|                  | yes          | 500       | $1 \cdot 10^{-4}$ | 1024      | –       | 0.1       | 30 min |

  

| Model            | Pre-trained? | dimension | learning rate     | ReVerb45K |         |           |      |
|------------------|--------------|-----------|-------------------|-----------|---------|-----------|------|
|                  |              |           |                   | batch     | dropout | N3 weight | time |
| NoENCODER_TUCKER | no           | 100       | $1 \cdot 10^{-3}$ | 512       | 0.4     | –         | 2.5h |
|                  | yes          | 300       | $3 \cdot 10^{-4}$ | 4096      | 0.3     | –         | 2.5h |
| NoENCODER_CONVE  | no           | 300       | $3 \cdot 10^{-4}$ | 512       | 0.3     | –         | 2h   |
|                  | yes          | 500       | $1 \cdot 10^{-4}$ | 2048      | 0.3     | –         | 2.5h |
| NoENCODER_5★E    | no           | 200       | $1 \cdot 10^{-3}$ | 2048      | –       | 0.3       | 3h   |
|                  | yes          | 200       | $1 \cdot 10^{-4}$ | 512       | –       | 0.1       | 3h   |
| GRU_TUCKER       | no           | 300       | $1 \cdot 10^{-3}$ | 512       | 0.4     | –         | 3h   |
|                  | yes          | 300       | $3 \cdot 10^{-4}$ | 2048      | 0.4     | –         | 3h   |
| GRU_CONVE        | no           | 300       | $1 \cdot 10^{-4}$ | 4096      | 0.3     | –         | 2h   |
|                  | yes          | 500       | $3 \cdot 10^{-4}$ | 2048      | 0.3     | –         | 2.5h |
| GRU_5★E          | no           | 500       | $3 \cdot 10^{-4}$ | 1024      | –       | 0.03      | 3h   |
|                  | yes          | 500       | $3 \cdot 10^{-4}$ | 2048      | –       | 0.1       | 3h   |

  

| Model            | Pre-trained? | dimension | learning rate     | FB15K237 |         |           |      |
|------------------|--------------|-----------|-------------------|----------|---------|-----------|------|
|                  |              |           |                   | batch    | dropout | N3 weight | time |
| NoENCODER_TUCKER | no           | 200       | $3 \cdot 10^{-4}$ | 1024     | 0.4     | –         | 9.5h |
|                  | yes          | 300       | $3 \cdot 10^{-5}$ | 2048     | 0.4     | –         | 9.5h |
| NoENCODER_CONVE  | no           | 300       | $3 \cdot 10^{-4}$ | 2048     | 0.3     | –         | 8.5h |
|                  | yes          | 500       | $3 \cdot 10^{-4}$ | 512      | 0.3     | –         | 9h   |
| NoENCODER_5★E    | no           | 500       | $1 \cdot 10^{-4}$ | 512      | –       | 0.3       | 12h  |
|                  | yes          | 500       | $1 \cdot 10^{-4}$ | 512      | –       | 0.3       | 12h  |
| GRU_TUCKER       | no           | 100       | $3 \cdot 10^{-4}$ | 512      | 0.4     | –         | 13h  |
|                  | yes          | 200       | $1 \cdot 10^{-4}$ | 1024     | 0.4     | –         | 13h  |
| GRU_CONVE        | no           | 300       | $3 \cdot 10^{-4}$ | 512      | 0.3     | –         | 11h  |
|                  | yes          | 500       | $3 \cdot 10^{-4}$ | 512      | 0.3     | –         | 12h  |
| GRU_5★E          | no           | 500       | $1 \cdot 10^{-4}$ | 1024     | –       | 0.1       | 24h  |
|                  | yes          | 500       | $3 \cdot 10^{-4}$ | 512      | –       | 0.1       | 24h  |

  

| Model            | Pre-trained? | dimension | learning rate     | WN18RR |         |           |      |
|------------------|--------------|-----------|-------------------|--------|---------|-----------|------|
|                  |              |           |                   | batch  | dropout | N3 weight | time |
| NoENCODER_TUCKER | no           | 100       | $1 \cdot 10^{-3}$ | 512    | 0.3     | –         | 7.5h |
|                  | yes          | 100       | $1 \cdot 10^{-3}$ | 512    | 0.3     | –         | 7.5h |
| NoENCODER_CONVE  | no           | 300       | $1 \cdot 10^{-3}$ | 512    | 0.3     | –         | 8h   |
|                  | yes          | 300       | $1 \cdot 10^{-3}$ | 512    | 0.3     | –         | 8h   |
| NoENCODER_5★E    | no           | 200       | $1 \cdot 10^{-3}$ | 512    | –       | 0.3       | 8h   |
|                  | yes          | 500       | $1 \cdot 10^{-3}$ | 1024   | –       | 0.3       | 8h   |
| GRU_TUCKER       | no           | 100       | $1 \cdot 10^{-3}$ | 512    | 0.3     | –         | 6h   |
|                  | yes          | 100       | $1 \cdot 10^{-3}$ | 1024   | 0.4     | –         | 6h   |
| GRU_CONVE        | no           | 300       | $1 \cdot 10^{-3}$ | 1024   | 0.3     | –         | 8.5h |
|                  | yes          | 500       | $1 \cdot 10^{-3}$ | 2048   | 0.3     | –         | 8.5h |
| GRU_5★E          | no           | 500       | $3 \cdot 10^{-4}$ | 512    | –       | 0.1       | 8.5h |
|                  | yes          | 500       | $1 \cdot 10^{-3}$ | 1024   | –       | 0.3       | 8.5h |

Table 7: Best hyperparameter setups and training time of best models for all datasets.
